# Supplementary material for: Partial Order-Disorder Transition Driving Closure of Band Gap: Example of Thermoelectric Clathrates
Source: arXiv:2009.11137 ancillary file (2020-09-23)
Supplement: Supplementary file 1 [file SM.pdf]

# Supplemental Material for "Partial Order-Disorder Transition Driving Closure of Band Gap: Example of Thermoelectric Clathrates"

Maria Troppenz[1],* Santiago Rigamonti[1], Jorge O. Sofo[2], and Claudia Draxl[1]
[1]*Institut für Physik und Iris Adlershof, Humboldt-Universität zu Berlin, zum Großen Windkanal 6, 12489, Berlin, Germany*
[2]*Department of Physics and Materials Research Institute, The Pennsylvania State University, University Park, Pennsylvania 16802, USA*

## I. COMPUTATIONAL DETAILS

The *ab-initio* calculations are performed with the full-potential all-electron density-functional-theory code `exciting` [1], using the exchange-correlation functional PBEsol [2]. Each structure is optimized by employing the same procedure as in Ref. [3]. To speed up convergence, we use the mixing algorithm of Ref. [4] for some structures. All energies are given with respect to the ground-state energy, $E_{\mathrm{GS}} = -39130343\,\mathrm{meV/atom}$. For the 44 computed $Ba_8Al_{16}Si_{30}$ configurations, 6 of them come from the ground-state search performed in Ref. [3], and 15 are obtained from a simulated-annealing technique. The latter are low-energy structures with energies less than 10 meV/atom above the GS, in order to capture a sufficiently large variety of configurations in this region.

## II. CANONICAL AVERAGE IN TERMS OF THE CONFIGURATIONAL DENSITY OF STATES

The expectation value of a configuration-dependent property $P_c$ at temperature $T$ is, in the canonical ensemble:

$$P_T = \frac{1}{Z_T}\sum_c P_c e^{-E_c/k_B T}. \tag{1}$$

The sum runs on the complete configuration space of the alloy. $Z_T$ is the canonical partition function $Z_T = \sum_c e^{-E_c/k_B T}$. In the configuration space, the energy $E_c$ for configuration $c$ is in the interval $[E_0, E_{max}]$, with $E_0$ the ground state energy and $E_{max}$ the maximum possible energy attained by a configuration. This interval can be partitioned in $M+1$ sub-intervals $\Delta_{E,i} \equiv [E_i, E_i + \Delta_i)$, with $E_i = E_{i-1} + \Delta_{i-1}$ and $E_{max} = E_M + \Delta_M$, and $i = 0$-$M$. In terms of these sub-intervals, we can write the summation in Eq. (1) as follows:

$$P_T = \frac{1}{Z_T}\sum_{i=0}^{M}\sum_{c\in S_i} P_c e^{-E_c/k_B T}. \tag{2}$$

Here, $S_i$ denotes the set of all configurations with energies in the sub-interval $\Delta_{E,i}$. Assuming that the interval widths $\Delta_i$ are not too large, one can approximate, for $c \in S_i$, $e^{-E_c/k_B T} \sim e^{-E_i/k_B T}$. Applying this to Eq. (2), we obtain

$$P_T = \frac{1}{Z_T}\sum_{i=0}^{M} N_i \langle P\rangle_i e^{-E_i/k_B T}. \tag{3}$$

Here, $\langle P\rangle_i = \sum_{c\in S_i} P_c/N_i$ is the average of $P_c$ in $S_i$, and $N_i$ is the number of configurations in $S_i$. It can be approximated as

$$N_i \sim \Delta_i g(E_i), \tag{4}$$

with $g(E)$ being the configurational density of states. Using this, we get:

$$P_T \simeq \frac{1}{Z_T}\sum_{i=0}^{M} \langle P\rangle_i \Delta_i g(E_i) e^{-E_i/k_B T}. \tag{5}$$

*Electronic address: `maria.troppenz@physik.hu-berlin.de`

In this work, we approximate the true means $\langle P\rangle_i$ by an estimate based on a random sampling of the configurational space. To summarize, there are two approximations made in passing from Eq.(1) to Eq.(5): the evaluation of the exponentials at $E_i$ and the estimate of the averages $\langle P\rangle_i$ on the sub-intervals.

## III. SYMMETRY-AVERAGED SPECTRAL FUNCTION

For the purpose of calculating the temperature-dependent band structure along the Γ-$M$ path, the symmetry-averaged spectral function is evaluated. This function is an average over 6 distinct Γ-$M$ directions, namely $(k_x, k_y, k_z) = (0.0, 0.5, 0.5)$, $(0.0, 0.5, -0.5)$, $(0.5, 0.0, 0.5)$, $(0.5, 0.0, -0.5)$, $(0.5, 0.5, 0.0)$, and $(0.5, -0.5, 0.0)$. For the ground state and a selected high-energy structure, the band structure along these directions, and the resulting symmetry-averaged spectral function are shown in Figs. 1(a) and (b), respectively. The symmetry-averaged spectral function for five configurations with intermediate energy (see labels above the panels) are shown in Fig. 2.

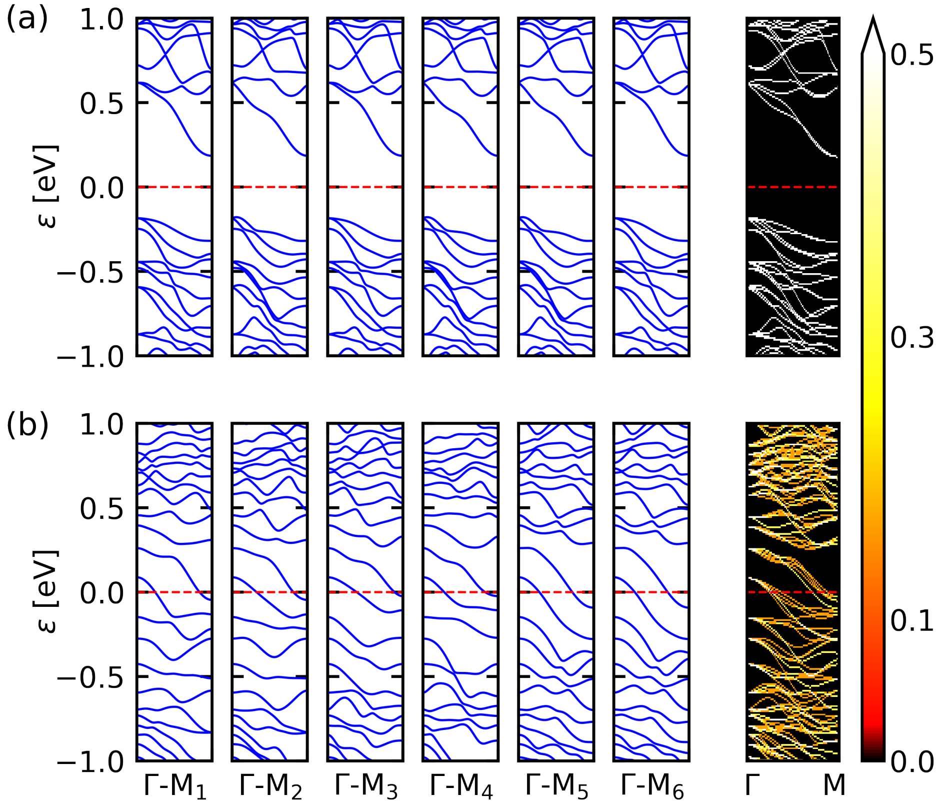


Supplementary Fig. 1: 6 distinct Γ-$M$ directions (left panels) and the symmetry-averaged spectral function (right panels) for (a) the ground state and (b) a high-energy configuration. Black corresponds to $A_c(\mathbf{k}, \epsilon) = 0$ and white to $A_c(\mathbf{k}, \epsilon) > 0.5$.

## IV. FINITE-TEMPERATURE SIMULATIONS

The finite-temperature simulations are carried out with the cluster-expansion package `CELL` [5, 6], using the cluster-expansion model of Ref. [3]. The converged configurational density-of-states $g(E)$ obtained from a Wang-Landau sampling is shown in Fig. 3. Using $g(E)$, the temperature-dependent electronic density of states (DOS) is obtained from a canonical-ensemble average as

$$\mathrm{DOS}_T(\epsilon) = \frac{1}{Z_T} \sum_i^M \langle \mathrm{DOS}(\epsilon)\rangle_i \, \Delta_i g(E_i) e^{-E_i/k_B T} \ . \tag{6}$$

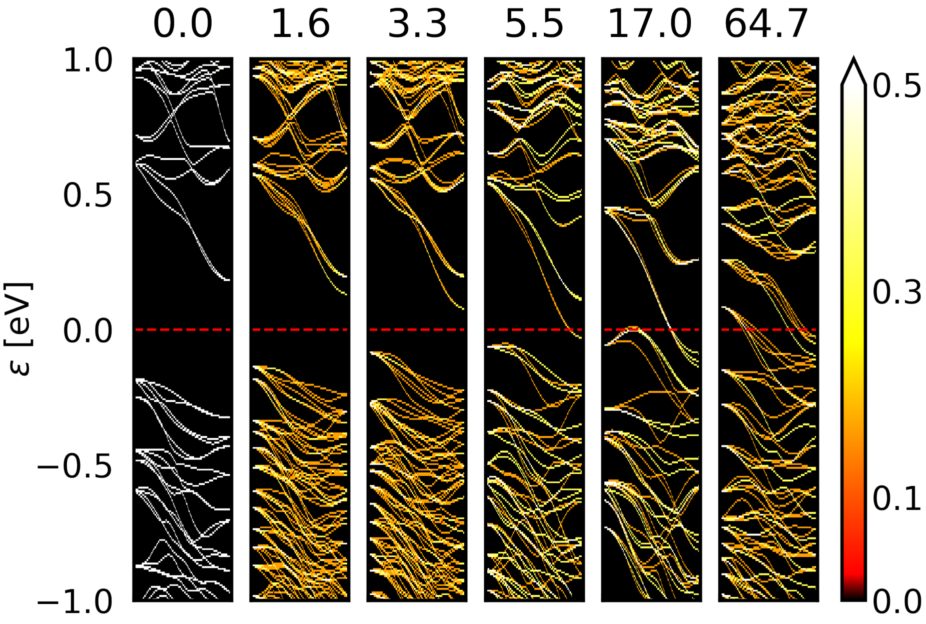


Supplementary Fig. 2: Symmetry-averaged spectral function of three semiconducting and two metallic configurations. The numbers on top of each panel indicate the total energy $E$ of the corresponding structure with respect to the ground state ($E$ in meV/atom).

Here, $\langle \mathrm{DOS}(\epsilon)\rangle_i = \sum_{c\in\Delta_{E_i}} \mathrm{DOS}_c(\epsilon)/n_i$ is the configuration-averaged DOS in the energy interval $\Delta_E = [E_i, E_i + \Delta_i)$, with $\Delta_i$ being the interval width. $n_i$ is the number of computed configurations in $\Delta_{E_i}$, while $\Delta_i g(E_i)$ is the total number of configurations in the same interval.

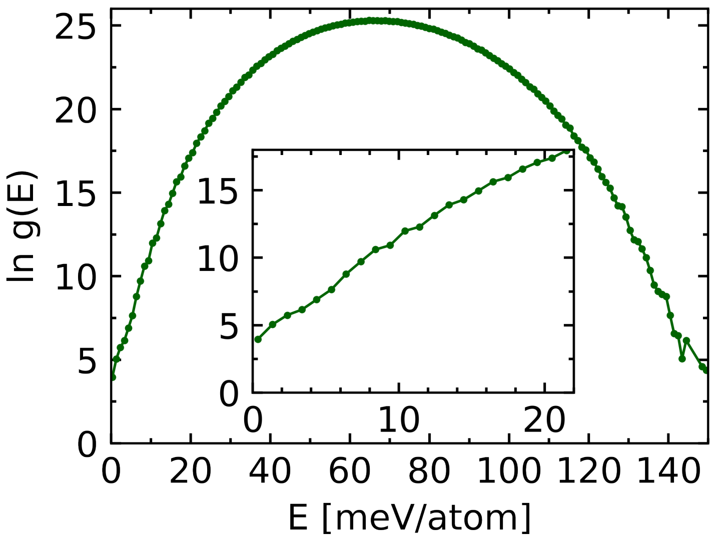


Supplementary Fig. 3: Normalized configurational density of states $g(16, E)$ obtained by the Wang-Landau method [7] for the single unit cell. The bin width of the energy histogram is 1 meV/atom. The sampling starts with the modification factor $f = e \approx 2.72$ and a flatness condition of 50% for the sampling histogram, successively improves $g(E)$ by lowering $f$ and increasing the flatness condition until the 27th (final) iteration with $f = 1.0000000149$ ($\ln f = 1.49 \cdot 10^{-8}$ ) and a flatness condition of 98%.

For the Metropolis Monte-Carlo (MC) simulations, we perform 10 million sampling steps for the unit cell and 80 million sampling steps for the $2 \times 2 \times 2$ supercell at every temperature. The first half of these sampling steps is

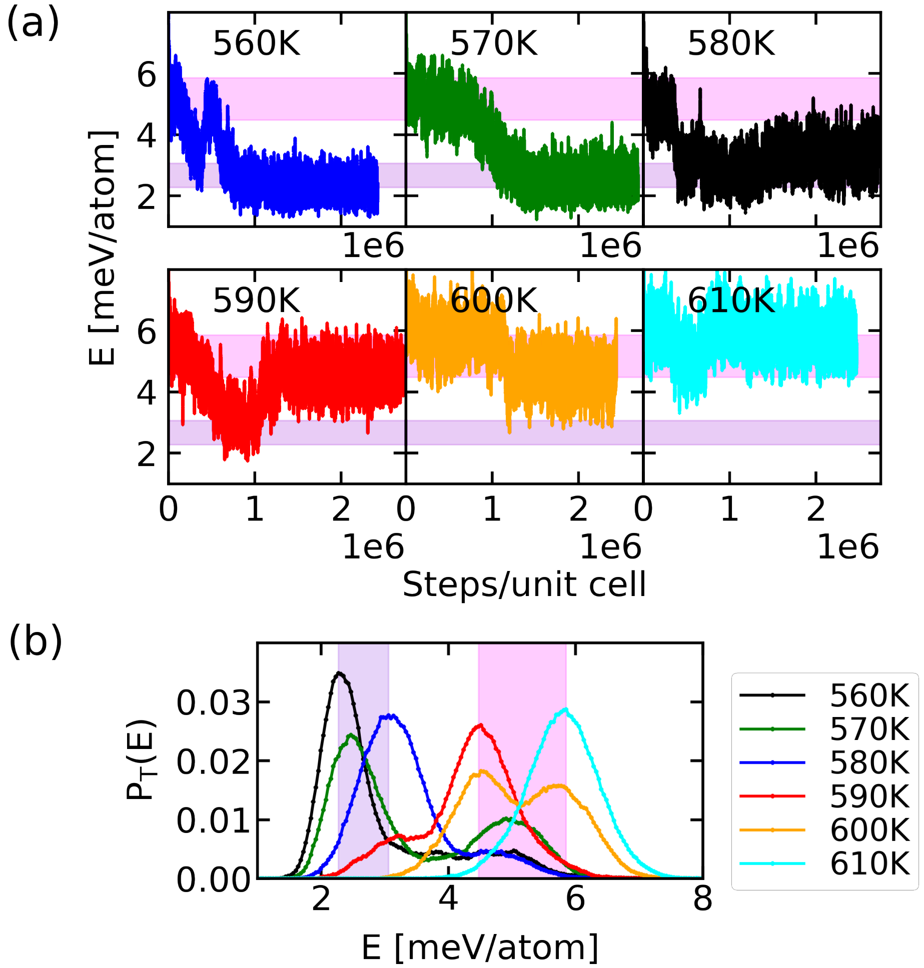


Supplementary Fig. 4: (a) Metropolis Monte-Carlo (MC) samplings in the $4 \times 4 \times 4$ supercell and (b) their canonical probability distributions, $P_T(E)$, for temperatures of 560 K, 570 K, 580 K, 590 K, 600 K, and 610 K. The low- and high-energy phase are indicated by the violet and magenta areas, respectively.

taken for equilibration, and the second half for averaging. For the $4 \times 4 \times 4$ supercell, we perform about 80 million sampling steps at every temperature. Here, the number of equilibration steps is determined for each temperature individually by analyzing its sampling trajectory (around 60 million steps for low temperatures and 5 million steps for high temperatures).

For the $4 \times 4 \times 4$ supercell, the estimate of the transition temperature $T_{tr}$, presented in Fig. 4(c) of the main manuscript, is obtained by an inspection of the MC trajectories and the canonical probability distributions for temperatures between 560 K and 610 K. As seen from the MC trajectories in Fig. 4(a), the system swaps between a low (violet) and high (magenta) energy phase, and finally remains in one of the phases for very long (*i.e.* a large number of MC steps). Their corresponding canonical probability distributions, that are depicted in Fig. 4(b), reveal a double-peak structure with peaks at the low- and the high-energy phase (phase coexistence). Below $T \leq 580$ K, the low-energy phase is preferred (the peak of $P_T(E)$ in this energy region is more pronounced), while, for $T \geq 590$ K, the high-energy phase is more favorable. This change is indicating the transition region. We take the mean value of these temperatures as an estimate for $T_{tr}$, *i.e.* $T_{tr} = 585$ K.

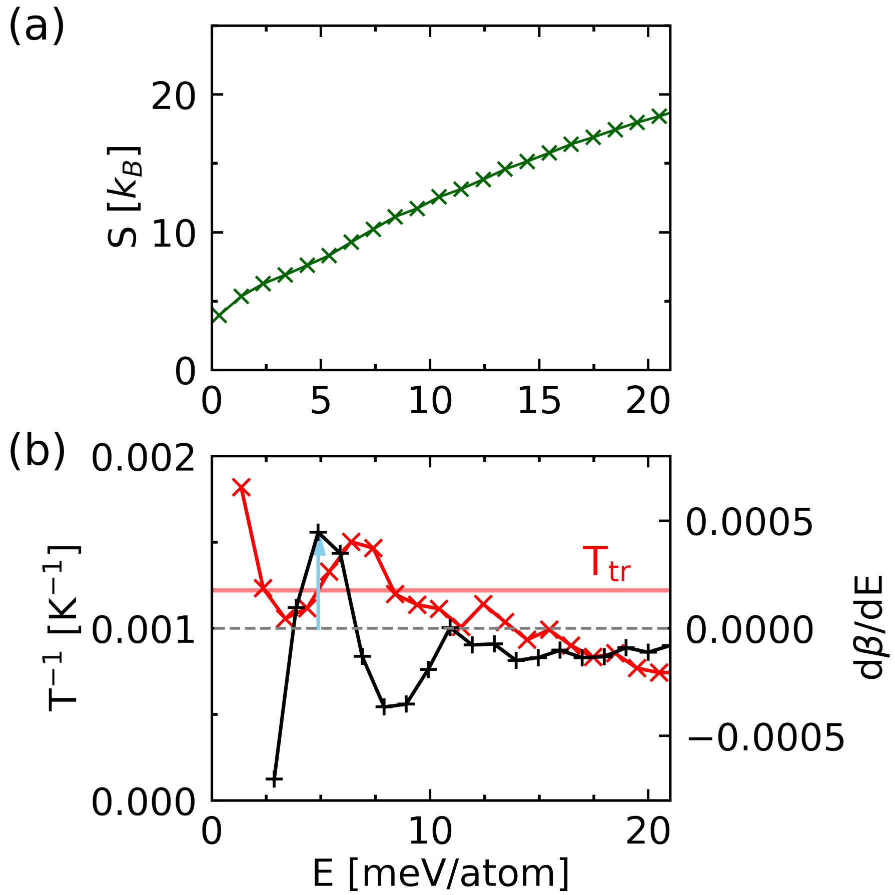


Supplementary Fig. 5: (a) Microcanonical entropy $S$ and (b) its energy derivatives versus total energy $E$. The first derivative, $T^{-1}(E) = \beta$, is shown in red (left axis) and the second derivative, $d\beta/dE$, in black (right axis). The inverse of the transition temperature for the unit cell $1/820\,\mathrm{K}^{-1} = 0.00122$, shown by the red horizontal line, matches the position of the inflection point of $\beta$.

## V. MICROCANONICAL ENTROPY

As a further verification that the partial order-disorder phase transition is a first-order phase transition, we examine the microcanonical entropy $S(E)$ and its derivatives in the microcanonical ensemble [8]. $S(E)$ is calculated as

$$S(E) = k_B \ln G(E) \tag{7}$$

and shown in Fig. 5(a). Here, the integrated density of states $G(E) = \int_{E_{\mathrm{GS}}}^{E} g(E')dE'$ is obtained by using $g(E)$ for the single unit cell. The first derivative of $S$ with respect to the energy $E$ is the inverse of the temperature $T^{-1}(E) = \beta = (dS/dE)_{N,p}$ (red solid line in Fig. 5(b)). It has an inflection point at the inverse of the transition temperature for the unit cell $1/T_{tr} = 1/820\,\mathrm{K}^{-1} = 0.00122$ (light-red horizontal line). The second derivative $d\beta/dE = d^2S/dE^2$ shown with the black solid line in Fig. 5(b), is positive at this inflection point (light blue arrow), thus suggesting that the phase transition is of first-order.

[1] A. Gulans, S. Kontur, C. Meisenbichler, D. Nabok, P. Pavone, S. Rigamonti, S. Sagmeister, U. Werner, and C. Draxl, Journal of Physics: Condensed Matter **26**, 363202 (2014).
[2] J. P. Perdew, A. Ruzsinszky, G. I. Csonka, O. A. Vydrov, G. E. Scuseria, L. A. Constantin, X. Zhon, and K. Burke, Phys. Rev. Lett. **100**, 136406 (2008).
[3] M. Troppenz, S. Rigamonti, and C. Draxl, Chem. Mater. **29**, 2414 (2017).

[4] J. Kim, A. Gulans, and C. Draxl, Electronic Structure **2**, 037001 (2020).
[5] S. Rigamonti *et al.*, `CELL`: a python package for cluster expansion with a focus on complex alloys, in preparation.
[6] `CELL` documentation: `https://sol.physik.hu-berlin.de/cell`.
[7] F. Wang and D. P. Landau, Physical Review Letters **86**, 2050 (2001).
[8] S. Schnabel, D. T. Seaton, D. P. Landau, and M. Bachmann, Phys. Rev. E **84**, 011127 (2011).
